# Supplementary material for: Full-Duplex Wideband mmWave Integrated Access and Backhaul with Low Resolution ADCs
Source: arXiv:2202.00566 source file (2022-02-06)
Supplement: Supplementary file 1 [file appendix.tex]

\appendices
\section{Derivation of LMMSE Precoder}
